# Supplementary material for: AegisAsync: Symbolic Async-Event Simulation for Risks in Python Asynchronous Programs
Source: arXiv:2610.18831 source file (2026-10-13)
Supplement: Supplementary file 1 [file appendix_bug_cases.tex]

%\FloatBarrier
\section{Case Studies}\label{app:bugcase}

This appendix presents representative source-confirmed findings with
behavioral PoC validation, complementing the aggregate results in
Table~\ref{tab:bug-poc-status}.
% We include one case from each detector family for which a PoC has been
% developed and reproduced: task lifetime, blocking operation,
% admission/fan-out, queue admission, missing timeout, and cancellation suppression.
% Each case summarizes the reported code pattern, the witness produced by
% {\tech}, and the observed runtime behavior.
We present three representative source-confirmed findings with behavioral PoC validation, covering blocking operation, admission/fan-out, and cancellation suppression. Each case summarizes the reported code pattern, the witness produced by {\tech}, and the observed runtime behavior.

%\input{sections/5-evaluation/case-study-1}

\input{sections/5-evaluation/case-study-2}

\input{sections/5-evaluation/case-study-3}

%\input{sections/5-evaluation/case-study-4}

%\input{sections/5-evaluation/case-study-5}

\input{sections/5-evaluation/case-study-6}
